# Supplementary material for: The network epidemiology of an Ebola epidemic
Source: arXiv:2111.08686 ancillary file (2021-11-16)
Supplement: Supplementary file 1 [file supplementary_material.pdf]

# Supplementary Information for The network epidemiology of an Ebola epidemic

**Laurent Hébert-Dufresne[1,2,3,4,*], Jean-Gabriel Young[2,3,5], Jamie Bedson[6], Laura Skrip[7,4], Danielle Pedi[8], Mohamed F. Jalloh[9], Bastian Raulier[3], Olivier Lapointe-Gagné[3], Amara Jambai[10], Antoine Allard[2,3,11], and Benjamin M. Althouse[4,12,13,†]**

[1]Department of Computer Science, University of Vermont, Burlington VT, USA
[2]Vermont Complex Systems Center, University of Vermont, Burlington VT, USA
[3]Département de physique, de génie physique et d'optique, Université Laval, Québec (Québec), Canada
[4]Institute for Disease Modeling, Global Health, Bill & Melinda Gates Foundation, Seattle WA, USA
[5]Department of Mathematics and Statistics, University of Vermont, Burlington VT, USA
[6]Independent Consultant, Seattle WA, USA
[7]School of Public Health, University of Liberia, Monrovia, Liberia
[8]Bill & Melinda Gates Foundation, Seattle, WA USA
[9]Division of Global Health Protection, Center for Global Health, CDC, Atlanta GA, USA
[10]Ministry of Health and Sanitation, Freetown, Sierra Leone
[11]Centre interdisciplinaire en modélisation mathématique, Université Laval, Québec (Québec), Canada
[12]University of Washington, Seattle WA, USA
[13]New Mexico State University, Las Cruces NM, USA
[*]laurent.hebert-dufresne@uvm.edu
[†]bma85@uw.edu

## ABSTRACT

This supplementary information document presents additional details on five fronts. (1) We describe the Sierra Leone Ebola Database. (2) We describe the Bayesian inference procedure used in the main text to infer distribution of secondary infections from outbreak sizes, and vice versa. (3) We summarize the Approximate Bayesian Computation method to infer summary statistics of epidemiological parameters and predict outbreak sizes from incidence time series. (4) We clarify the formulation of our network model under different parametrization for the distributions of secondary infections. (5) We present an agent-based metapopulation model to explore and support our conclusion that reductions in EVD cases were largely driven by reduction in migration and introduction of EVD in new regions, and not by reduction of secondary infections.

# Contents


**1 Data Modeling Community Engagement in Health Emergencies and The Sierra Leone Ebola Database 3**

**2 Backward prediction: From outbreak sizes (meso) to secondary infections (micro) 4**

2.1 Problem statement . . . . . . 4

2.2 Inference . . . . . . 4

2.3 Priors . . . . . . 5

Poisson • Exponential • Power law • Power law with an exponential cutoff • Negative binomial • Semiparametric prior

2.4 Model selection . . . . . . 6

**3 Forward prediction: From secondary infections (micro) to outbreak sizes (meso) 7**

**4 From incidence curves (macro) to outbreak sizes (meso) 8**

4.1 Problem statement . . . . . . 8

4.2 Sampling the posterior distribution of the epidemiological parameters . . . . . . 8

Distributions for the number of secondary cases and for serial intervals • Simulating the time evolution of cumulative incidence at the population level • Sampling procedure

4.3 Sampling the posterior outbreak size distribution . . . . . . 9

4.4 Sensitivity analysis . . . . . . 10

**5 Families of network models 13**

5.1 One parameter families . . . . . . 13

Poisson • Exponential • Power law distribution

5.2 Two parameter families . . . . . . 14

Power law distribution with exponential cutoff • Negative binomial distribution

5.3 Semiparametric families . . . . . . 15

**6 Simulation of a metapopulation model 17**

**References 19**

# 1 Data Modeling Community Engagement in Health Emergencies and The Sierra Leone Ebola Database

This project is part of a broader initiative - "Data Modeling Community Engagement in Health Emergencies" – that is focused on interrogating the relationship between community engagement and related behavior change and Ebola transmission during the 2014 – 2016 Ebola outbreak in Sierra Leone. The primary objective of the project is to contribute to efforts focused on quantifying and testing analytical behavior change disease modeling using the extensive empirical data gathered during the Ebola response in Sierra Leone. The project was a collaboration between the Bill and Melinda Gates Foundation, the Institute for Disease Modeling and researchers and practitioners from a range of institutions.

The Ebola Outbreak in West Africa was a unique health emergency, both in terms of the scale and patterns of transmission. The international biomedical and community engagement response from the Government of Sierra Leone and the international community was unprecedented in both size and scope, generating an historically unique set of both epidemiological and community-level behavior change intervention and longitudinal data on the knowledge, attitudes and practices of communities.

A core component of this project, including for this paper, was working with the Government of Sierra Leone's Ministry of Health and Sanitation (MoHS) and the US Centers for Disease Control and Prevention to access epidemiological data contained within the recently completed Sierra Leone Ebola Database (SLED)[1].

The SLED initiative is an ambitious project to consolidate data from 30 government and international agencies collected by the MoHS's Emergency Control Center over the course of the Sierra Leone Ebola outbreak. SLED consists of data collected by the national reporting hotline and district alert lines, case investigations, laboratory sample testing, clinical management and safe and dignified burial records. While the primary objective of the SLED project is to identify the graves of those that died during the Ebola outbreak as a part of the SLED Family Reunification Project, the database also acts as a lasting post epidemic resource for researchers in Sierra Leone and in other locations. The "Data Modeling Community Engagement in Health Emergencies" team were pleased to participate as one of the pilot research projects utilizing the SLED data. Participation as a pilot enabled the SLED team to test and revise a process for ethical and efficient access and ensure the viability of the database as a lasting resource for researchers into the future[1,2].

## 2 Backward prediction: From outbreak sizes (meso) to secondary infections (micro)

In this section we describe the procedure followed to generate parts of the results presented in Fig. 2 of the main text.

### 2.1 Problem statement

We observe $N$ outbreaks of sizes $X_1,...,X_N$. We think of these outbreaks as the disconnected components of a graph, whose edges represent transmission events (we do not model inter-cluster spread). We wish to infer the excess degree distribution of this graph, or in other words the distribution of secondary infections, using only the outbreak sizes. Making this inference requires a model for the network of contacts. We use a maximally agnostic model and assume that the graph is fully random—except for variations in the degrees, since we know that heterogeneity is a major determinant of epidemiological outcome. This means that our model is a random graph with fixed degree distribution, known as the configuration model.

### 2.2 Inference

The inference problem we want to solves connects component sizes to secondary infections: given a series of outbreak sizes, we want to determine the distribution of the number of secondary infections.

Probability generating functions (PGFs) allow us to bridge the two mathematically. For the purpose of inference we can think of PGF as blackboxes that allow us to take a distribution of secondary cases, $\{u_n\}_{n=0,..,\infty}$ as input and compute the distribution of component sizes $\{h_n\}_{n=0,...,\infty}$.

To determine if a distribution of secondary cases match the outbreak data, we assign a likelihood to the data by first computing the predicted distribution outbreak sizes $\{h_n\}$ (with PGFs) and then evaluating:

$$\log P(X|h) = \sum_{i=1}^{N} \log h_{X_i} \equiv \sum_{n=0}^{\infty} m_n \log h_n, \tag{1}$$

where $m_n$ is the number of outbreak of size $n$, i.e., $m_n = \sum_j 1_{\{X_i=n\}}$. This likelihood is valid when the outbreak sizes are independent from one another. This assumption is true in the configuration model we have used to model the data and hence reasonable to make here. More realistic models could include correlations.

Finding the distribution of secondary infections most likely to have led to the observed data is a matter of maximizing $P(X|h)$ over some space of distributions. Since this space is large and we do not have much data to inform our choice, we'll use a parametric approach and assume that $\{u_j\}$ comes from some known family, for example a Poisson distribution parameterized by its mean $\lambda$. Finding a good distribution then boils down to finding the best member of the family (e.g., the best $\lambda$). We can readily solve this second problem in most cases.

To account for uncertainty we adopt a Bayesian approach and focus on the posterior distribution of model parameters $\theta$, given by

$$P(\theta|X) \propto P(X|\theta)P(\theta) \tag{2}$$

where $P(\theta)$ is a prior over the parameters and where $P(X|\theta)$ denotes the likelihood of the outbreak size shown in Eq. (1).

The specific prior depends on the choice of model; see Sec. 2.3 where we describe the parameters chosen for each family. We select these priors by using domain knowledge about the relevant parameters, such as the mean number of secondary case $R_0$, and doing prior-predictive check to ensure that the *a priori* predictions are sensible, following best Bayesian practice[3].

To estimate the parameters $\theta$ given $X$, we minimize the inverse of the logarithm of the joint probability $P(\theta,X)$,

$$\Sigma = -\log P(X|\theta) - \log P(\theta) \tag{3}$$

over all values of $\theta$ using gradient descent, which gives us a maximum a posteriori (MAP) estimate $\hat{\theta}$ of the parameters. The posterior distribution of many of the models considered here is somewhat rugged, so whenever a global optima is difficult to find, we run the minimization algorithm starting from 500 initial conditions drawn at random from the prior distribution.

In all cases, we fit a semiparametric version of the model where the first $d$ degrees of liberty of the distribution of secondary cases – $\boldsymbol{u}(d) = \{u_0,...,u_{d-1}\}$ – are treated as free parameters also, to be inferred jointly with the parameters of the "base" family of distributions (see Sec. 5.3). This gives the model some flexibility while keeping the number of parameters small. In practice this means that the parameters $\theta$ consists of (a) one or two parameters for the base family, (b) $d-1$ coefficients $\boldsymbol{u}$ and (c) the number of free parameters $d$. Since $d$ is discrete, in practice we run the minimization described above for several values of $d$ and select the best MAP estimator.

### 2.3 Priors

We consider five base families of models for the distribution of secondary cases: Poisson, exponential, power law, power law with an exponential cutoff, and negative binomial. The specific form of their probability mass functions and associated probability generation functions are given in Sec. 5 below.

#### 2.3.1 Poisson

The parameter of the Poisson distribution is its mean, $R_0$. We use a log-normal distribution on this parameter:

$$P(R_0) = \frac{1}{R_0\sigma\sqrt{2\pi}} \exp\left(-\frac{(\ln R_0 - \mu)^2}{2\sigma^2}\right) \qquad R_0 > 0, \tag{4}$$

where $\mu$ is a location parameter and $\sigma$ a shape parameter. In all our simulations with this prior we use $\mu = \ln 2 - 1/2, \sigma = 1$ which ensures our prior on $R_0$ is positive, of mean 2, and gives most of its mass to the range $[0,5]$ while allowing for significant larger values of $R_0$.

#### 2.3.2 Exponential

The parameter of the exponential distribution is a characteristic scale $\kappa$, which can be roughly thought of as a shifted mean. Thus, for the prior we use the same log-normal distribution with $\mu = \ln 2 - 1/2, \sigma = 1$ as before. Since $R_0$ scales like $\kappa$ with a slight offset, the prior on $R_0$ is very similar to the prior on $\kappa$ even given the transformation of variable.

#### 2.3.3 Power law

The parameter of the power law distribution is a scaling exponent $\tau$ which must be greater than 2 (otherwise the PGFs cannot be computed due to divergences in the moments). Based on prior-predictive tests, we opt for a uniform prior in the range $[2,5]$. This prior on $\tau$ implies a non-uniform prior on $R_0$ with most of its mass near smaller values of $R_0$, but with much larger values of $R_0$ still allowed, much like the log-normal.

#### 2.3.4 Power law with an exponential cutoff

The power law with an exponential cutoff has two parameters: a scaling exponent $\tau$ and a characteristic scale $\kappa > 0$. Due to the exponential cutoff, $\tau$ it not bounded from below at $\tau = 2$. We use independent priors on $\tau$ and $\kappa$ such that $P(\tau,\kappa) = P(\tau)P(\kappa)$. Prior-predictive tests show that a uniform prior on $\tau$ on the range $[-3,3]$ is reasonable, and the usual log-normal prior on $\kappa$ works, again with $\mu = \ln 2 - 1/2, \sigma = 1$.

#### 2.3.5 Negative binomial

The negative binomial has two parameters. We use a parametrization in terms of its mean $R_0$ and a dispersion parameter $k > 0$, and choose independent priors again. Since lower values of $k$ are associated with higher variance in the distribution of secondary contacts, and since we expect such variances in our data, we a truncated exponential prior

$$P(k) = \frac{1}{m}\frac{e^{-k/m}}{1-e^{-U/m}} \qquad k \in [0,U] \tag{5}$$

where $m$ is a pseudo-mean and $u = 10$ is an upper bound. For $R_0$ we choose the usual log-normal prior with $\mu = \ln 2 - 1/2, \sigma = 1$.

#### 2.3.6 Semiparametric prior

The semiparametric version of each model has several additional parameters: the number of degrees of freedom $d$ and the $d$ first entries of the probability mass function, $\boldsymbol{u}(d) = \{u_0, ..., u_{d-1}\}$. We parametrize the complete prior as

$$P(\theta, \boldsymbol{u}(d), d) = P(\theta)P(\boldsymbol{u}(d)|d)P(d). \tag{6}$$

where $P(\theta)$ is the priors of the "base family" of distributions. Noting that $u_0, ..., d_{d-1}$ must sum to 1 or less, we choose as $P(\boldsymbol{u}(d)|d)$ a *projection* of the uniform distribution over the regular $d$-simplex. More precisely, we imagine drawing a random point in this simplex dropping one of the entries of the resulting vector by choosing it uniformly at random from all entries. Since the volume of the regular $d$-simplex is $1/d!$, and since there are $d$ ways to obtain the same vector by dropping one of

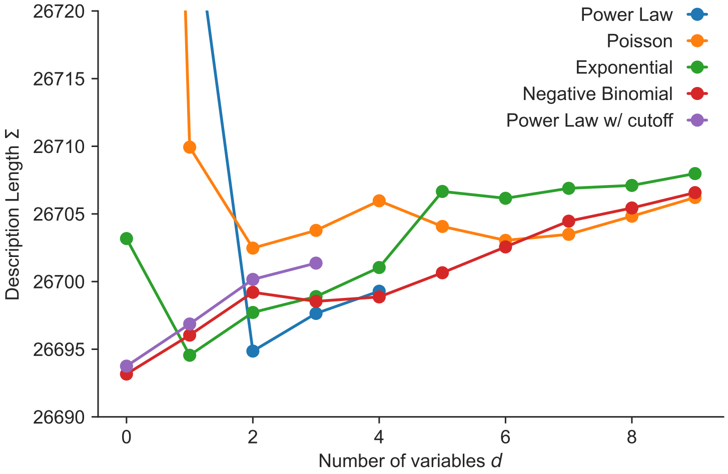


**Figure 1.** Description length of the best fit for several values of $d$ and all models. The prior $P(\boldsymbol{u},d)$ regularizes the inference and favors sparser models even if the added degrees of liberty would lead to a more accurate model of the data $X$. The best fits have the following description lengths: $\Sigma^* = 26693$ (Negative binomial, $d = 0$), $\Sigma^* = 26694$ (Power law with cutoff, $d = 0$), $\Sigma^* = 26697$ (Exponential, $d = 1$), $\Sigma^* = 26699$ (Power law, $d = 2$), $\Sigma^* = 26707$ (Poisson, $d = 2$).

the $d$ coordinates, we obtain $P(\boldsymbol{u}(d)|d) = d! \times \frac{1}{d} \times d = d!$ as the density function of the prior. For $P(d)$ we use the maximum entropy distribution on the non-negative integers, under the constraint that the mean be finite. It corresponds to the geometric distribution $P(d) = (1-p)^d p$. We set $p = 0.95$, reflecting our prior assumption that very few degrees of freedoms should be needed to explain the data.

Note that in the rest of this document (inference, model selection), we use $\theta$ to refer to the parameters of the family of distribution jointly with $\{u_1, ..., u_{d-1}\}$ and $d$.

## 2.4 Model selection

To select among the many possible model for the data we resort to the minimum description length (MDL) criterion[4,5], since the Bayes factor cannot be computed in closed form. The MDL criterion is derived by interpreting $\Sigma$ as information-theoretic quantity. Indeed, $\Sigma$ in Eq. (3) can be viewed as the information cost associated with communicating the data $X$ to a receiver aware of the prior and likelihood. The first term, $-\log P(X|\theta)$, is the information cost associated with sending the data $X$ to a receiver that assumes that the outbreak sizes were generated independently and identically at random from the distribution of small components $\{h_k\}$ implied by the model, when its parameter equals $\theta$. The second term, $-\log P(\theta)$, can be viewed as the cost of sending the value of a parameter $\theta$ to a receiver that assumes that they were drawn from the prior $P(\theta)$. Thus $\Sigma$ is the total information cost associated with sending the data and parameters, or in other words the *description length* of the data under the model. In particular, the minimum description length (MDL) found by maximizing $\Sigma$ is the cost of sending the data when we find its best possible description under a given model.

This information criterion automatically penalizes model that overfit to the observed data, as complex models able to fit the data very well by maximizing $\log P(X|\theta)$ will generally require very complicated priors $P(\theta)$[4], that incur high information costs $-\log P(\theta)$. Hence, by selecting the model and fit associated with the smallest MDL, we balance accuracy and complexity.

## 3 Forward prediction: From secondary infections (micro) to outbreak sizes (meso)

In this section we describe the procedure followed to generate parts of the results presented in Fig. 2 of the main text.

Forward prediction aims to forecast the distribution of outbreak sizes from contact tracing information. This is a standard calculation that can be accomplished by solving Equations (1)-(4) of the main text, for a distribution $\{u_n\}$ estimated from contact tracing efforts.

That said, contact tracing data are notoriously noisy, so we add uncertainty to the simulation shown in Fig. 2. First, we estimate $u_0$, the probability that a case leads to no further infection, because it is unknown in our data (the data do not distinguish between no secondary infections and no contact tracing efforts). We do this with the Bayesian method presented in Section. 2.

Second, to account for the fact that the distribution of secondary cases may contain measurement errors, we generate $10,000$ new distributions of secondary infections $\{(\tilde{u}_i\}$ from a Dirichlet distribution whose probability density function is

$$P(\tilde{\boldsymbol{u}}) \propto \prod_i \tilde{u}_i^{\alpha_i}. \tag{7}$$

We set $\alpha_i = C(u_i + \varepsilon)$, which ensure that the expected distribution is the measured one, while including deviations from the mean. Here, $\varepsilon = 10^{-14}$ is added to ensure that $\alpha_i > 0$ for all $i$, while $C$ controls the size of those deviations. We choose $C = 100$ in the simulation, which means that the distribution are fairly concentrated around $\{u_i\}$.

For each possible distribution of secondary cases, we solve Eqs (1)-(4) and obtain a distribution of outbreak sizes. Finally, to simulate finite size effects, we generated a sample of $14,297$ outbreaks from each of those distributions. Thus we were able to estimate, for each outbreak size $i$, the *range* of the probability that an outbreaks is of size $i$.

## 4 From incidence curves (macro) to outbreak sizes (meso)

In this section we describe the procedure followed to generate the results presented in Fig. 3 pf the main text.

### 4.1 Problem statement

We observe one single time series of cumulative incidence over a 90-day period starting from the first confirmed EVD case. We note this time series $\{I_t\}_{t=1,...,90}$. Our two main objectives are:

1. to infer the four parameters of our model for the time evolution of cumulative incidence at the population level ($R_0$, $k$, $\sigma$, $\alpha$; see Sec. 4.2) from $\{I_t\}_{t=1,...,90}$ using Approximate Bayesian Computation (ABC)[6,7];

2. to use the posterior distribution for $R_0$ and $k$ to obtain the posterior outbreak size distribution using a probability generating functions formalism (PGF; see Sec. 4.3)[8,9].

### 4.2 Sampling the posterior distribution of the epidemiological parameters

In what follows, we describe the ABC procedure used to estimate the posterior distribution of the parameters $R_0$, $k$, $\sigma$, and $\alpha$.

#### *4.2.1 Distributions for the number of secondary cases and for serial intervals*

We assume that the number $n$ of secondary cases per infected individual is distributed according to a negative binomial distribution

$$P(n|R_0,k) = \frac{\Gamma(n+k)}{\Gamma(n+1)\Gamma(k)}\left(\frac{R_0}{R_0+k}\right)^n\left(1-\frac{R_0}{R_0+k}\right)^k \tag{8}$$

of mean $R_0 > 0$ and dispersion $k > 0$. We model the interval between the time an individual gets infected and the time it infects one of its neighbors, the serial interval $t$, is distributed according to a gamma distribution[7]

$$Q(t|\sigma,\alpha) = \frac{\alpha^\alpha}{\sigma^\alpha\Gamma(\alpha)}t^{\alpha-1}\mathrm{e}^{-\frac{\alpha t}{\sigma}} \tag{9}$$

of mean $\sigma > 0$ and shape $\alpha > 0$.

#### *4.2.2 Simulating the time evolution of cumulative incidence at the population level*

Assuming that a value has been assigned to $R_0$, $k$, $\sigma$ and $\alpha$, the simulation goes as follows.

1. A single index case $i = 1$ becomes infectious on day 1 (“patient zero”).

   (a) Set $x_i = 1$

   (b) Draw the number $n_i$ of secondary cases caused by this individual from $P(n_i|R_0,k)$.

   (c) Assign a unique number to each of the $n_i$ new secondary cases, and add these numbers to the list of new secondary cases $L$.

2. For an individual $j$ in $L$:

   (a) Draw the serial interval $t_j$ from $Q(t_j|\sigma,\alpha)$ and set $x_j = x_l + t_j$, where $l$ is the individual who infected $j$.

   (b) If $x_j > 90$, proceed to step 2(e).

   (c) Draw the number $n_j$ of secondary cases caused by individual $j$ from $P(n_j|R_0,k)$.

   (d) Assign a unique number to each of the $n_j$ new secondary cases, and add these numbers to the list of new secondary cases $L$.

   (e) Remove $j$ from $L$.

3. Repeat step 2 until $L$ is empty, then proceed to step 4.
4. Compute the simulated time series of cumulative incidence $\{X_t\}_{t=1,\ldots,90}$ as

$$X_t = \sum_m \mathbb{1}(x_m \leq t) \ ,$$

for $t = 1, \ldots, 90$ where $\mathbb{1}(\cdot)$ is the indicator function.

#### 4.2.3 Sampling procedure

A sample of the posterior distribution for $R_0$, $k$, $\sigma$ and $\alpha$ is obtained via the following ABC procedure inspired from that of Riou & Althaus[7].

1. Assign a value to $R_0$, $k$, $\sigma$ and $\alpha$ by sampling the prior marginal distributions

$$\begin{aligned} R_0 &\sim \mathrm{Uniform}(0.01, 5) \\ k &\sim \mathrm{Loguniform}(10^{-4}, 10) \\ \sigma &\sim \mathrm{Uniform}(0, 75) \\ \alpha &\sim \mathrm{Uniform}(0, 25) \ . \end{aligned}$$

2. Simulate a time series of cumulative incidence $\{X_t\}_{t=1,\ldots,90}$ with the procedure presented in Sec. 4.2.2, and compute the relative error

$$\varepsilon_d = \frac{|X_d - I_d|}{I_d}$$

for $d$ = 15, 30, 45, 60, 75 and 90.

3. If $\varepsilon_d < 0.3$ for all $d$ considered at the previous step, add the values assigned to $R_0$, $k$, $\sigma$ and $\alpha$ at step 1 to the sample of the posterior distribution.

### 4.3 Sampling the posterior outbreak size distribution

Having sampled the posterior distribution for $R_0$, $k$, $\sigma$ and $\alpha$, we are now in a position to compute the posterior outbreak size distribution using a probability generating functions formalism[8–10]. The two PGFs required by this formalism, $G_1(x)$ and $G_0(x)$, are provided by Eqs. (35)–(38).

The only unknown parameter remaining—the probability that the primary case of a new cluster does not transmit the disease at all, $p_0$—is fixed by asking that the expected number of secondary cases caused directly by the primary case, $z$, is as close to $R_0$ as possible. This requirement is written mathematically as

$$p_0 = \max\left\{0, 1 - \frac{1}{z_0}\right\} \ , \tag{10}$$

where $z_0$ is defined in Eq. (38).

A general expression for the outbreak size distribution $\{\pi(s)\}_{s=1,2,3,\ldots}$ is provided by Newman[9], which we adapt here to our notation

$$\pi(s) = \begin{cases} \dfrac{p_0}{G_0(a)} & s = 1 \\ \dfrac{z}{(s-1)!\, G_0(a)} \left[\dfrac{d^{s-2}}{dx^{s-2}} \left[G_1(x)\right]^s\right]_{x=0} & s > 1 \ , \end{cases} \tag{11}$$

where $a$ is smallest value in $(0, 1)$ satisfying the equation[8]

$$a = G_1(a) \ . \tag{12}$$

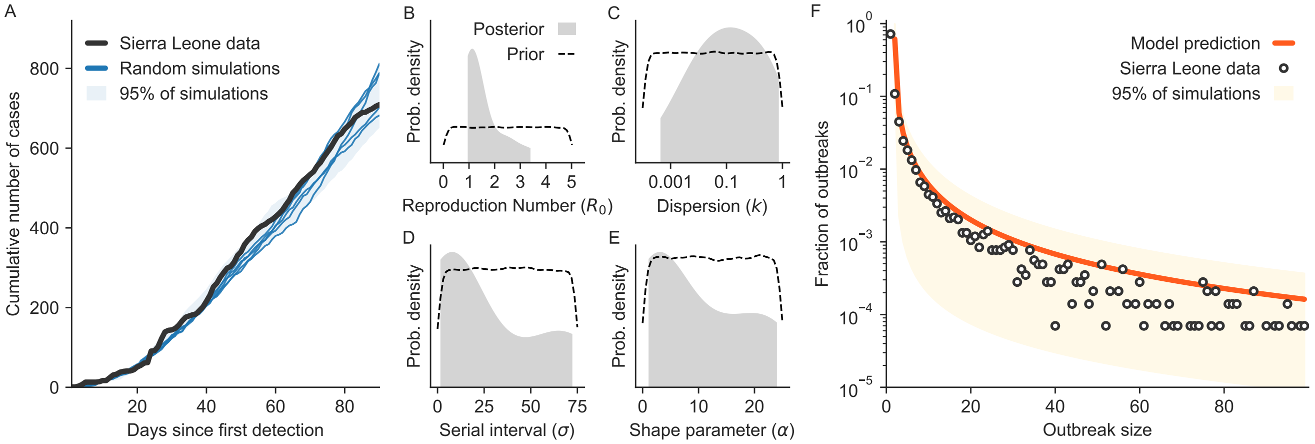


**Figure 2.** Same as Fig. 3 in the main text, but with $\epsilon_d < 0.15$ for $d$ =10, 20, 30, 40, 50 ,60, 70, 80 and 90.

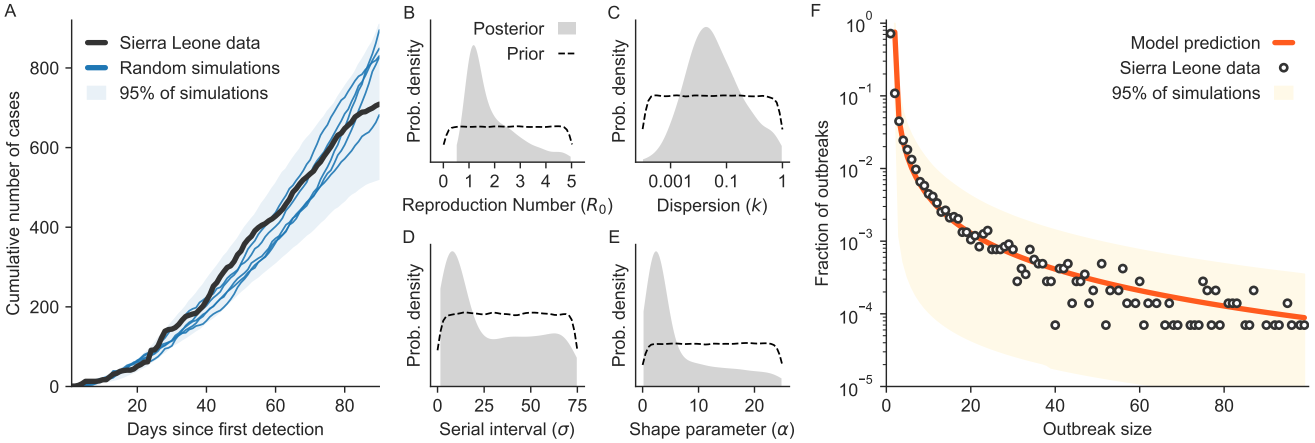


**Figure 3.** Same as Fig. 3 in the main text, but with $\epsilon_d < 0.30$ for $d$ =10, 20, 30, 40, 50, 60, 70, 80 and 90.

Substituting Eq. (35) into Eq. (11) yields

$$\pi(s) = \begin{cases} \dfrac{p_0}{G_0(a)} & s = 1 \\ \dfrac{(1-p_0)R_0 z_0}{G_0(a)} \dfrac{\Gamma(sk+s-2)}{\Gamma(s)\Gamma(sk)} \left(\dfrac{R_0}{R_0+k}\right)^{s-2} \left(\dfrac{k}{R_0+k}\right)^{sk} & s > 1\,. \end{cases} \tag{13}$$

With Eq. (13) in hand, we now can sample the posterior outbreak size distribution: for each tuple $(R_0, k, \sigma, \alpha)$ identified in Sec. 4.2.3, we compute a sample of the posterior outbreak size distribution $\{\pi(s)\}_{s=1,\ldots,s_{\max}}$ using Eq. (13) and with $s_{\max} = 100$.

## 4.4 Sensitivity analysis

Figures 2–9 show different versions of Fig. 3 in the main text obtained with the ABC procedure for various tolerances $\epsilon_d$ and various time windows $d$ (see Sec. 4.2.3).

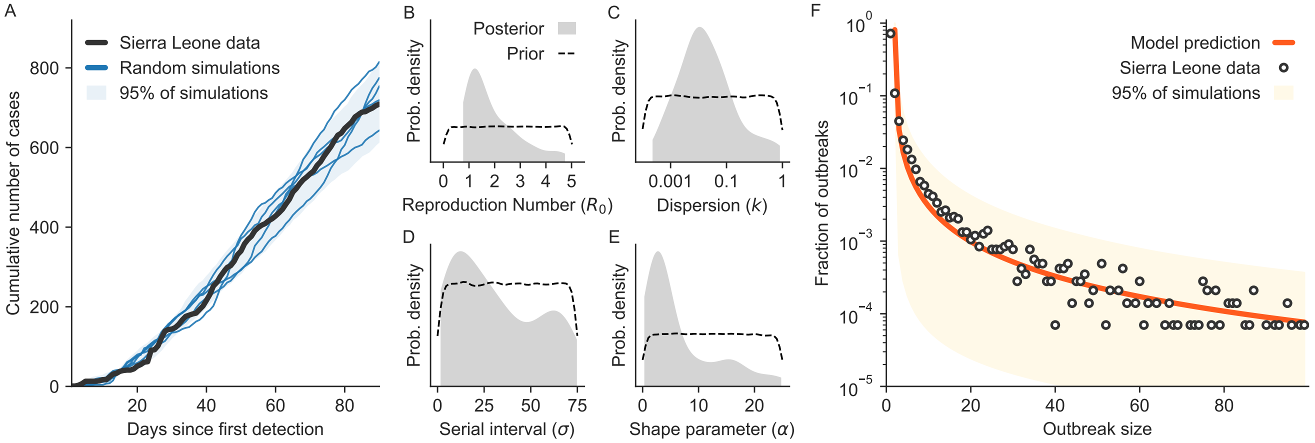


**Figure 4.** Same as Fig. 3 in the main text, but with $\varepsilon_d < 0.15$ for $d =$15, 30, 45, 60, 75 and 90.

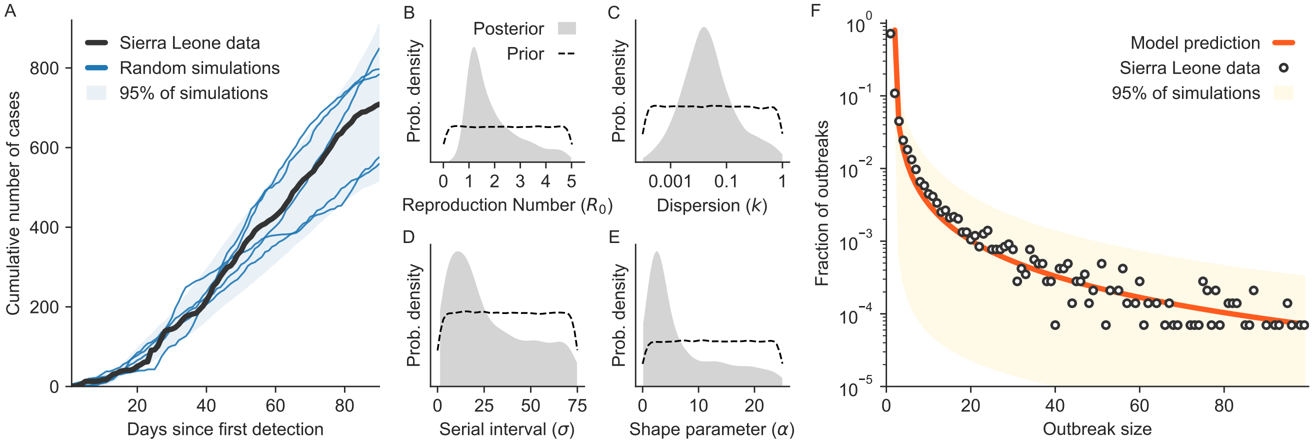


**Figure 5.** Same as Fig. 3 in the main text ($\varepsilon_d < 0.30$ for $d =$15, 30, 45, 60, 75 and 90). Reproduced here for the sake of comparison.

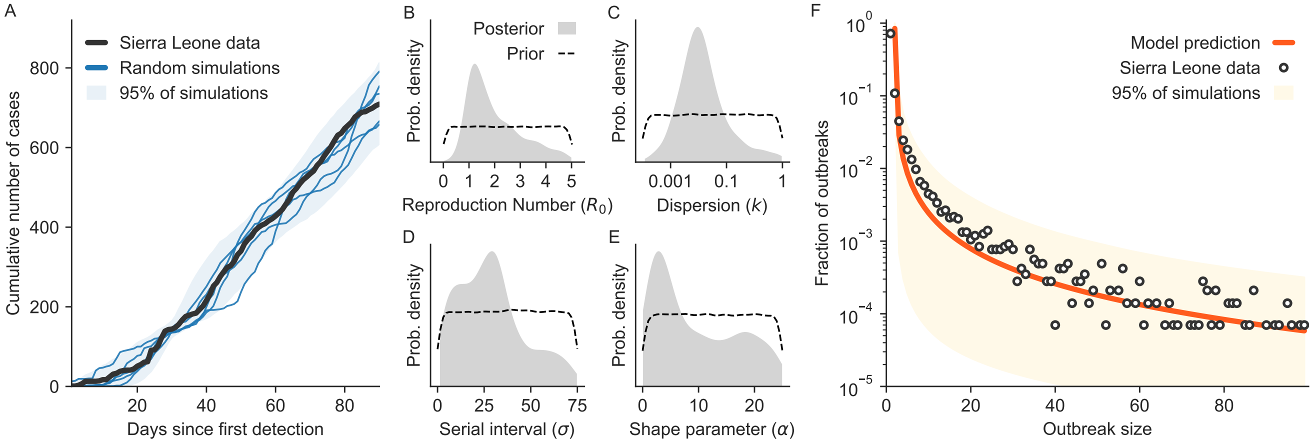


**Figure 6.** Same as Fig. 3 in the main text, but with $\varepsilon_d < 0.15$ for $d =$30, 60 and 90.

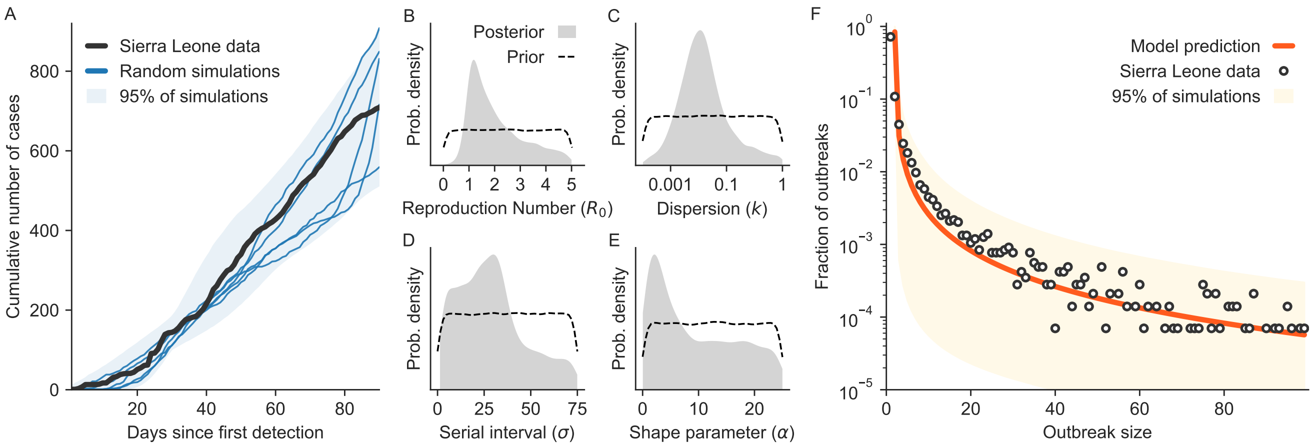


**Figure 7.** Same as Fig. 3 in the main text, but with $\varepsilon_d < 0.30$ for $d$ =30, 60 and 90.

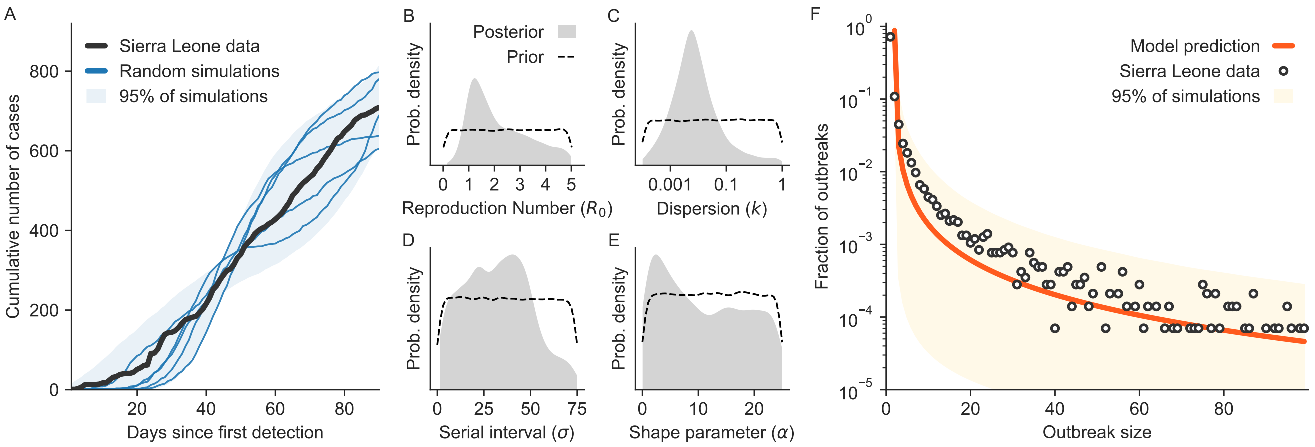


**Figure 8.** Same as Fig. 3 in the main text, but with $\varepsilon_d < 0.15$ for $d$ =45 and 90.

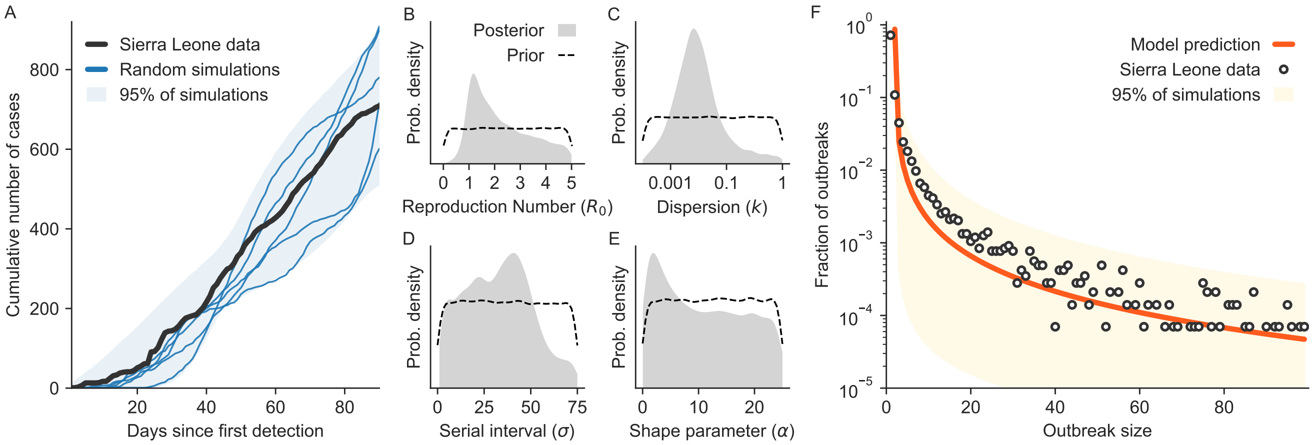


**Figure 9.** Same as Fig. 3 in the main text, but with $\varepsilon_d < 0.30$ for $d$ =45 and 90.

## 5 Families of network models

We consider the following parametric families distributions for the distribution of the number of secondary infections.

### 5.1 One parameter families

#### 5.1.1 Poisson

The probability $u_n$ that the number of secondary infection is $n$ for this family of models is given by

$$u_n = \frac{R_0^n}{n!} e^{-R_0}, \qquad n \geq 0, \tag{14}$$

where $R_0$ is the mean number of secondary infection.

The generating functions can be computed as

$$G_1(x) = \sum_{n=0}^{\infty} u_n x^n = e^{R_0(x-1)} \tag{15}$$

$$G_0(x) = \sum_{n=0}^{\infty} p_n x^n = \frac{z}{R_0}\left[e^{R_0(x-1)} - 1\right] + 1 \tag{16}$$

where $z$ is the mean of $\{p_n\}$ defined by $z = G_0'(1)$. Taking the series expansion of $G_0(x)$ in terms of $x$ reveals that

$$G_0(x) = 1 - \frac{z}{R_0} + \frac{ze^{-R_0}}{R_0}\left[1 + \Omega(x)\right] \tag{17}$$

where $\Omega(x)$ denotes terms that are bounded from below by $x$. Since the terms independent of $x$ are in fact $p_0$, we can parametrize $G_0(x)$ directly in terms of $p_0$, using

$$z = R_0 \frac{(1-p_0)}{1-e^{-R_0}}, \tag{18}$$

and subsequently replacing $z$ by this expression in $G_0(x)$. This expression is more useful to us since the value of $p_0$ is fixed by the data in our case study: it is the number of outbreak of size 1, namely the fraction of infected individuals that never cause a secondary infection.

#### 5.1.2 Exponential

We consider a discrete exponential distribution. The probability $u_n$ that the number of secondary infection is $n$ for this family of models is given by

$$u_n = (1 - e^{-1/\kappa})e^{-n/\kappa}, \qquad n \geq 0. \tag{19}$$

The parameter $\kappa$ is a characteristic scale but we note that it is related to $R_0$, the mean of the distribution, by

$$R_0 = \frac{e^{-1/\kappa}}{(1 - e^{-1/\kappa})}. \tag{20}$$

The generating functions have closed forms:

$$G_1(x) = \frac{(1 - e^{-1/\kappa})}{(1 - xe^{-1/\kappa})} \tag{21}$$

$$G_0(x) = \frac{z(1 - e^{-1/\kappa})}{e^{-1/\kappa}} \log \frac{(1 - e^{-1/\kappa})}{(1 - xe^{-1/\kappa})} + 1 \tag{22}$$

where $z$ is the mean of $\{p_n\}$ defined by $z = G_0'(1)$. If we want to parametrize $G_0(x)$ in terms of $p_0$ instead, we find:

$$z = (p_0 - 1)\frac{e^{-1/\kappa}}{(1 - e^{-1/\kappa})\log(1 - e^{-1/\kappa})}. \tag{23}$$

### 5.1.3 Power law distribution

We consider a power law distribution with infinite support, shifted so that it assigns some probability mass to case where there are no secondary infections. The probability $u_n$ that the number of secondary infection is $n$ for this family of models is given by

$$u_n = \frac{(n+1)^{-\tau}}{\zeta(\tau)}, \qquad n \geq 0, \tag{24}$$

where $\zeta(\tau) = \sum_{n=1}^{\infty} \frac{1}{\tau^n}$ is Riemann's zeta function. The parameter $\tau > 2$ is a scaling exponent but we note that it is related to $R_0$, the mean of the distribution, by

$$R_0 = \frac{\zeta(\tau-1)}{\zeta(\tau)} - 1. \tag{25}$$

The generating functions have the closed forms:

$$G_1(x) = \frac{1}{x}\frac{\mathrm{Li}_\tau(x)}{\zeta(\tau)} \tag{26}$$

$$G_0(x) = \frac{z}{\zeta(\tau)}\left[\mathrm{Li}_{\tau+1}(x) - \zeta(\tau+1)\right] + 1 \tag{27}$$

and the relationship between $z$ and $p_0$ is:

$$z = (1-p_0)\frac{\zeta(\tau)}{\zeta(\tau+1)}. \tag{28}$$

## 5.2 Two parameter families

### 5.2.1 Power law distribution with exponential cutoff

This is the same model as before in Sec. 5.1.3, but now with an added cutoff parameter to dampen the power law behavior in the tail. The probability $u_n$ that the number of secondary infection is $n$ for this family of models is given by

$$u_n = \frac{(n+1)^{-\tau} e^{-(n+1)/\kappa}}{\mathrm{Li}_\tau(e^{-1/\kappa})}, \qquad n \geq 0. \tag{29}$$

where $\kappa$ is a characteristic scale for the cutoff and $\tau$ is a scaling exponent. The exponent $\tau$ is no longer constrained and can take value in $\mathbb{R}$, but we need to have $\kappa > 0$. These parameters are related to $R_0$ by

$$R_0 = \frac{1}{e^{-1/\kappa}}\left[\frac{\mathrm{Li}_{\tau-1}(e^{-1/\kappa})}{\mathrm{Li}_\tau(e^{-1/\kappa})} - 1\right] \tag{30}$$

The distribution admits the following closed form for the generating functions:

$$G_1(x) = \frac{1}{x}\frac{\mathrm{Li}_\tau(xe^{-1/\kappa})}{\mathrm{Li}_\tau(e^{-1/\kappa})} \tag{31}$$

$$G_0(x) = \frac{z}{\mathrm{Li}_\tau(e^{-1/\kappa})}\left[\mathrm{Li}_{\tau+1}(xe^{-1/\kappa}) - \mathrm{Li}_{\tau+1}(e^{-1/\kappa})\right] + 1 \tag{32}$$

If we want to parametrize $G_0(x)$ in terms of $p_0$ instead, we have:

$$z = (1-p_0)\frac{\mathrm{Li}_\tau(e^{-1/\kappa})}{\mathrm{Li}_{\tau+1}(e^{-1/\kappa})}. \tag{33}$$

### 5.2.2 Negative binomial distribution

We consider a discrete negative binomial distribution. The probability $u_n$ that the number of secondary infection is $n$ for this family of models is given by

$$u_n = \frac{\Gamma(n+k)}{\Gamma(n+1)\Gamma(k)}\left(\frac{xR_0}{R_0+k}\right)^n \left(1 - \frac{R_0}{R_0+k}\right)^k, \qquad n \geq 0, \tag{34}$$

where $R_0 > 0$ is the average number of secondary cases and $k > 0$ is the dispersion parameter.

The distribution admits the following generating functions in closed forms:

$$G_1(x) = \sum_{n=0}^{\infty} u_n x^n = \sum_{n=0}^{\infty} \frac{\Gamma(n+k)}{\Gamma(n+1)\Gamma(k)} \left(\frac{xR_0}{R_0+k}\right)^n \left(1 - \frac{R_0}{R_0+k}\right)^k = \left[1 + \frac{R_0}{k}(1-x)\right]^{-k} \tag{35}$$

$$G_0(x) = \sum_{n=0}^{\infty} p_n x^n = p_0 + (1-p_0)\left[A \int G_1(x)dx + B\right] = \begin{cases} p_0 + (1-p_0)\dfrac{1 - \left[1 - \dfrac{R_0 x}{R_0+k}\right]^{1-k}}{1 - \left[\dfrac{k}{R_0+k}\right]^{1-k}} & k \neq 1 \\[2ex] p_0 + (1-p_0)\left[1 - \dfrac{\ln\left[1 + R_0(1-x)\right]}{\ln\left[1+R_0\right]}\right] & k = 1\ , \end{cases} \tag{36}$$

where the constants $A$ and $B$ are chosen such that $G_0(1) = 1$ and $G_0(0) = p_0 \in (0,1)$. The mean of the distribution generated by $G_0(x)$, $\{p_n\}$, is then

$$z = \sum_{n=0}^{\infty} n p_n = \left.\frac{dG_0(x)}{dx}\right|_{x=1} = (1-p_0)R_0 z_0 \tag{37}$$

where we defined

$$z_0 = \begin{cases} \dfrac{(1-k)}{k}\left[\left(\dfrac{k}{R_0+k}\right)^{k-1} - 1\right]^{-1} & k \neq 1 \\[2ex] \dfrac{1}{\ln\left[1+R_0\right]} & k = 1\ . \end{cases} \tag{38}$$

### 5.3 Semiparametric families

For every model family considered above, we can easily consider a semiparametric variant where $u_0, u_1, ..., u_{d-1}$ are treated as parameters and where $u_d, u_{d+1}, ...$ follow the parametric distribution up to a rescaling factor. This technique gives us a bit more of flexibility while ensuring that we do not overfit by introducing too many parameters.

We obtain the generating functions for a semiparametric distribution as follows. We denote by $\{\tilde{u}_n\}$ the distribution of secondary infections generated by the known probability generating function $\tilde{G}_1(x) = \sum \tilde{u}_n x^n$ which we wish to expand to a semiparametric form. We now want $G_0(x)$ and $G_1(x)$ for this semiparametric distribution:

$$\left\{u_0, ...u_{d-1}, \frac{1-\omega}{1-\tilde{\omega}}\tilde{u}_d, \frac{1-\omega}{1-\tilde{\omega}}\tilde{u}_{d+1}, ....\right\} \tag{39}$$

where the constants

$$\omega := \sum_{n=0}^{d-1} u_n \leq 1 \tag{40}$$

$$\tilde{\omega} := \sum_{n=0}^{d-1} \tilde{u}_n \leq 1 \tag{41}$$

$$\tag{42}$$

ensure its normalization. For the sake of brevity we'll write these constants as

$$\eta = \frac{1-\omega}{1-\tilde{\omega}}. \tag{43}$$

Using the fact that PGFs are formal power series, we can write $G_1(x)$ directly as

$$G_1(x) = \eta \tilde{G}_1(x) - \eta \sum_{n=0}^{d-1} \tilde{u}_n x^n + \sum_{n=0}^{d-1} u_n x^n. \tag{44}$$

by subtracting the spurious terms from $\tilde{G}_1(x)$ and adding the new free parameters $\{u_0, ..., u_{d-1}\}$. Supposing that we have computer code to calculate $\tilde{G}_1(x)$ in closed form, this equation lets us compute $G_1(x)$ in $O(d)$ additional steps.

The tricky part is finding $G_0(x)$. To do so we use the relationship $G_0(x) = z \int G_1(x)dx$ where $z$ is the mean generated by $G_0(x)$.

$$G_0(x) = z\left[\eta \int \tilde{G}_1(x)dx - \eta \sum_{n=0}^{d-1} \frac{\tilde{u}_n x^{n+1}}{n+1} + \sum_{n=0}^{d-1} \frac{u_n x^{n+1}}{n+1}\right] - C \tag{45}$$

Where $C$ is a constant of integration. Now, supposing that we have already calculated $\tilde{G}_0(x) := \tilde{z} \int \tilde{G}_1(x)dx$ for the parametric distribution, we can write this integral as

$$G_0(x) = z\left[\frac{1}{\tilde{z}}\eta \tilde{G}_0(x) - \eta \sum_{n=0}^{d-1} \frac{\tilde{u}_n x^{n+1}}{n+1} + \sum_{n=0}^{d-1} \frac{u_n x^{n+1}}{n+1}\right] - C. \tag{46}$$

To set $C$ we use the normalization condition $G_0(1) = 1$ and the fact that $\tilde{G}_0(x)$ is normalized also, which gives

$$C = z\left[\frac{1}{\tilde{z}}\eta - \eta \sum_{n=0}^{d-1} \frac{\tilde{u}_n}{n+1} + \sum_{n=0}^{d-1} \frac{u_n}{n+1}\right] - 1. \tag{47}$$

Thus we have

$$G_0(x) = z\left[\frac{\eta}{\tilde{z}}\left(\tilde{G}_0(x) - 1\right) - \eta \sum_{n=0}^{d-1} \frac{\tilde{u}_n \left(x^{n+1} - 1\right)}{n+1} + \sum_{n=0}^{d-1} \frac{u_n \left(x^{n+1} - 1\right)}{n+1}\right] + 1. \tag{48}$$

Again, supposing that we have computer code to calculate $\tilde{G}_0(x)$ in closed form, this equation lets us compute $G_0(x)$ in $O(d)$ additional steps.

To re-parametrize $G_0(x)$ in terms of $p_0$, we isolate the $O(1)$ terms and find

$$G_0(x) = 1 + \frac{z}{\tilde{z}}\eta(\tilde{p}_0 - 1) + z\eta \sum_{n=0}^{d-1} \frac{\tilde{u}_n}{n+1} - z\sum_{n=0}^{d-1} \frac{u_n}{n+1} + \Omega(x) \tag{49}$$

which gives

$$p_0 = 1 + \frac{z}{\tilde{z}}\eta(\tilde{p}_0 - 1) + z\eta \sum_{n=0}^{d-1} \frac{\tilde{u}_n}{n+1} - z\sum_{n=0}^{d-1} \frac{u_n}{n+1} \tag{50}$$

This sets $z$ as

$$z = (1 - p_0)\left[\eta \frac{(1 - \tilde{p}_0)}{\tilde{z}(\tilde{p}_0)} + \sum_{n=0}^{d-1} \frac{u_n - \eta \tilde{u}_n}{n+1}\right]^{-1} \tag{51}$$

Note that this equation depends on $\tilde{p}_0 = 1$, but its does not matter since changing $1 - \tilde{p}_0$ changes $\tilde{z}(\tilde{p}_0)$ in proportion. Thus we choose the arbitrary value $\tilde{p}_0 = 0$ when computing this equation.

## 6 Simulation of a metapopulation model

One of the key conclusion of our work is that reductions in introduction of EVD in new regions was likely a more significant driver than (unobserved) changes in the distribution of secondary infections per case. We wish to explore this conclusion further using an agent-based model on a metapopulation structure.

To compare the effects of an intervention reducing per-contact transmission probability to an intervention reducing migration of EVD to new communities, we developed a stochastic metapopulation model simulated using a Gillespie stochastic simulation algorithm[11] with the Binomial Tau leap approximation (BTL)[12]. BTL was chosen here for efficiency, computational speed and to avoid negative population sizes[12,13].

Briefly, we simulate $N$ villages with population sizes from 3000 to 100,000 drawn from a power law distribution with exponent -2.8 (based on rough unpublished estimates). Within each village, we assume dynamics follow a susceptible-exposed-infectious-recovered framework with latent period of 14 days, infectious period of 14 days, and disease-induced mortality of 50%[14]. Individuals move between patches at various rates, with active EVD infection reducing migration by 50%. We assume villages are connected to their 2-nearest neighbors as well as 35%, random, long-range connections to other villages.

We consider two interventions and a no-intervention control: 1) reducing the per-contact transmission probability by some percentage $\rho_T$, and 2) removing a percentage, $\rho_M$ of movement connections. We explore intervention effects from 5% to 95% by 10% intervals and perform 100 simulations at each value of the intervention effect. The main outcome explored was changes to the epidemic curve between the two interventions and control, as well as limiting the proportion of villages reached.

Results are presented in Fig. 10 and support two important conclusions. (i) Incidence curves alone do not help distinguish the mechanisms of intervention. (ii) The fact that 25% of Sierra Leone chiefdoms remained unaffected is more consistent with a model of reduction in migration, where 50% of model runs protect at least 25% of regions. Conversely, a model intervention on transmission alone protects 25% of regions in only 2% of simulations.

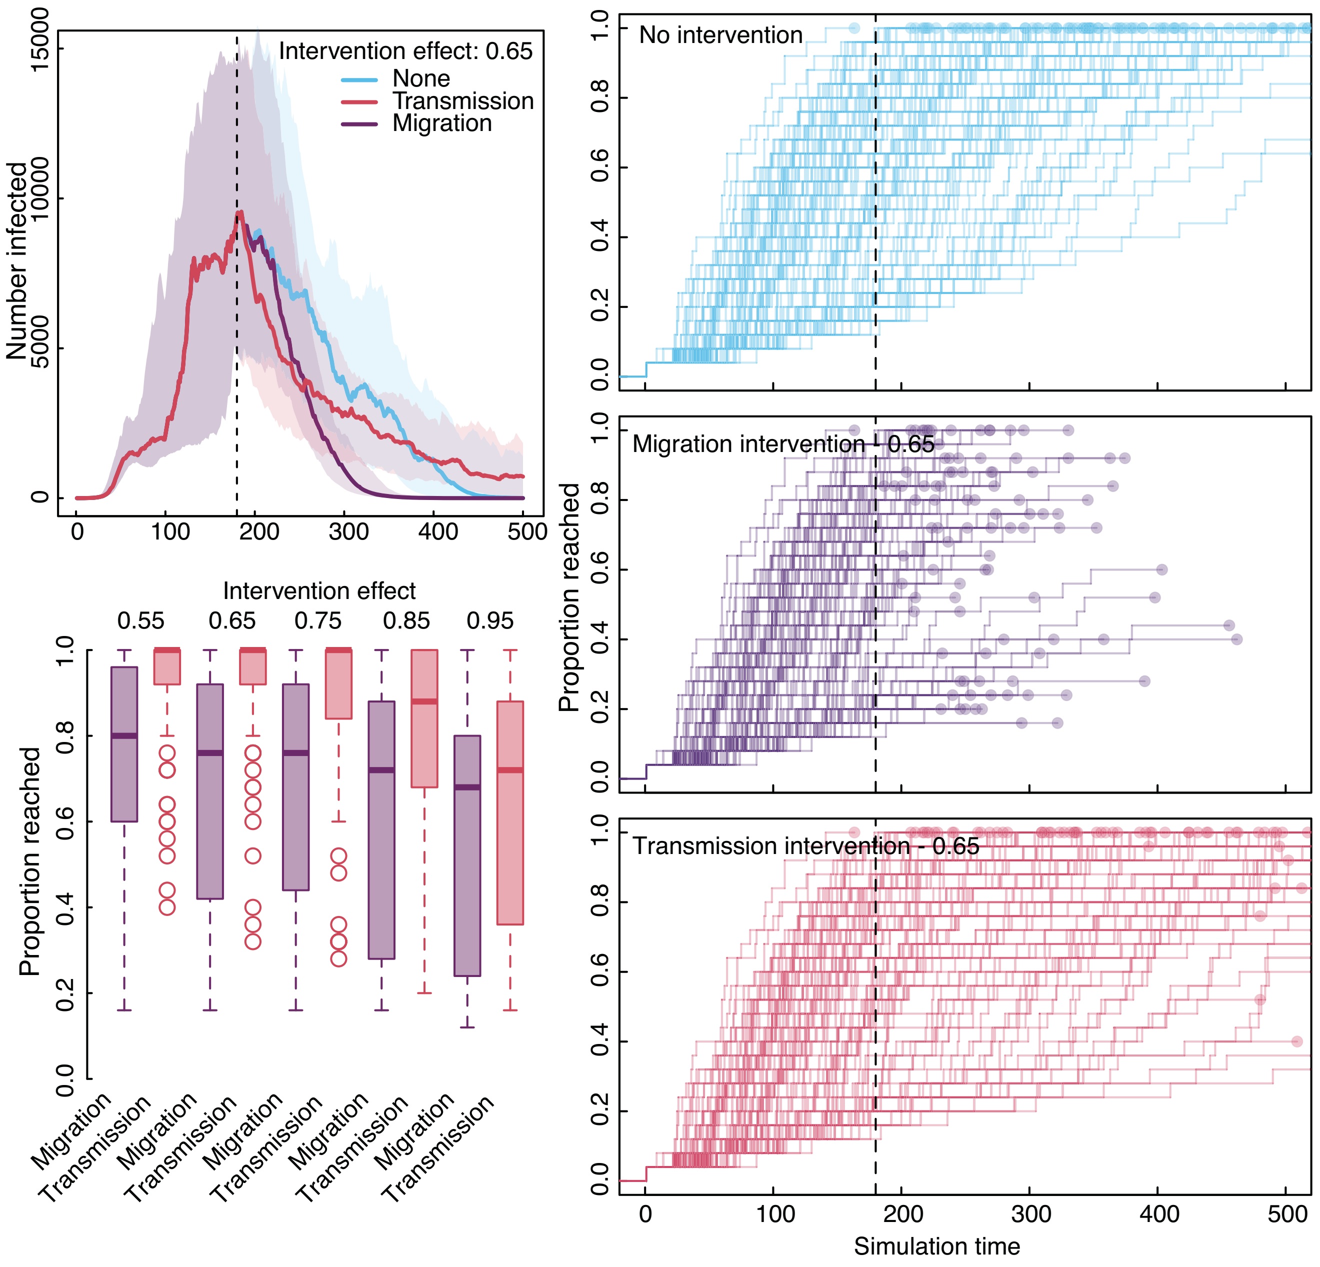


**Figure 10.** **Summary of metapopulation model results.** Figure summarizes runs of the metapopulation model with two interventions: reductions in the per contact transmission probability ("transmission intervention") and reductions in the movement of individuals to new communities ("migration intervention"). Upper left panel shows the number infected by day of the epidemic with no intervention (blue), transmission (red), and migration intervention (purple). Interventions were started on day 180 (dashed lines). Note the similarity in the case reductions between transmission and migration interventions. Right hand panels show the proportion of communities reached for no intervention (top, blue) and migration and transmission interventions (middle, purple; bottom, red, respectively). Note that migration interventions reduce the proportion of communities reached, while transmission does not as compared to no intervention. Bottom left panel compares the proportion of communities reached across intervention effects (0.55, 0.65, 0.75, 0.85, and 0.95) comparing migration to transmission interventions (purple and red, respectively). As intervention effects increase, the proportion of communities reached goes down.

## References


1. Agnihotri, S. *et al.* Building the Sierra Leone Ebola Database: organization and characteristics of data systematically collected during 2014-2015 Ebola epidemic. *Annals Epidemiol.* (2021).
2. Gorina, Y. *et al.* Ensuring ethical data access: the Sierra Leone Ebola Database (SLED) model. *Annals epidemiology* **46**, 1–4 (2020).
3. Gelman, A., Carlin, J. B., Stern, H. S. & Rubin, D. B. *Bayesian Data Analysis* (Chapman and Hall/CRC, 2013), 3rd edn.
4. Grünwald, P. D. *The Minimum Description Length Principle* (MIT Press, 2007).
5. MacKay, D. J. C. *Information Theory, Inference and Learning Algorithms* (Cambridge University Press, 2003), 1st edn.
6. Sunnåker, M. *et al.* Approximate Bayesian Computation. *PLOS Comput. Biol.* **9**, e1002803, DOI: 10.1371/journal.pcbi.1002803 (2013).
7. Riou, J. & Althaus, C. L. Pattern of early human-to-human transmission of Wuhan 2019 novel coronavirus (2019-nCoV), December 2019 to January 2020. *Eurosurveillance* **25**, 2000058, DOI: 10.2807/1560-7917.ES.2020.25.4.2000058 (2020).
8. Newman, M. E. J., Strogatz, S. H. & Watts, D. J. Random graphs with arbitrary degree distributions and their applications. *Phys. Rev. E* **64**, 026118, DOI: 10.1103/PhysRevE.64.026118 (2001).
9. Newman, M. E. J. Component sizes in networks with arbitrary degree distributions. *Phys. Rev. E* **76**, 045101, DOI: 10.1103/PhysRevE.76.045101 (2007).
10. Hébert-Dufresne, L., Althouse, B. M., Scarpino, S. V. & Allard, A. Beyond R0: heterogeneity in secondary infections and probabilistic epidemic forecasting. *J. R. Soc. Interface* **17**, 20200393, DOI: 10.1098/rsif.2020.0393 (2020).
11. Gillespie, D. Exact stochastic simulation of coupled chemical-reactions. In *Abstracts of Papers of the American Chemical Society*, vol. 173, 128–128 (1977).
12. Chatterjee, A., Vlachos, D. G. & Katsoulakis, M. A. Binomial distribution based tau-leap accelerated stochastic simulation. *J Chem Phys* **122**, 024112, DOI: 10.1063/1.1833357 (2005).
13. Pineda-Krch, M. GillespieSSA: Implementing the stochastic simulation algorithm in R. *J. Stat. Softw.* **25**, 1–18 (2008).
14. Lamontagne, F. *et al.* Evidence-based guidelines for supportive care of patients with Ebola virus disease. *The Lancet* **391**, 700–708 (2018).
